# Supplementary material for: Non-Gaussian tail in the force distribution: A hallmark of correlated disorder in the host media of elastic objects
Source: arXiv:2007.03089 source file (2020-07-06)
Supplement: Supplementary file 1 [file Supplementary_material.pdf]

## Supplementary Note 1

In the case of a superconductor with correlated pinning centers generated on cleaving the samples, strong fluctuations of the first-neighbor distances has been proposed as the fingerprint of a gel-like phase of vortices.[47] In the opposite scale of long-range vortex density fluctuations, some of us reported on the vortex structure nucleated in the cuprate superconductor $Bi_2Sr_2CaCu_2O_{8+\delta}$ with point and correlated pinning centers being hyperuniform at the sample surface.[46] A very recent study reveals disordered vortex structures observed in several pnictides and conventional superconductors seem also to be hyperuniform.[60] Hyperuniformity is a topological property of a state of matter characterized by strongly-reduced long-wavelength density fluctuations entailing an algebraically decaying structure factor for small wave-vectors. According to our study,[46] vortex structures nucleated in samples with a random distribution of point pins are theoretically expected to present hyperuniform structural properties. However, in the particular case of correlated pinning centers generated by columnar defecs (CD), no hyperuniform vortex structures are theoretically expected. Even though, the experimentally measured decay of the structure factor on decreasing $q$ in these samples is consistent with the structure being hyperuniform. We interpreted this apparent discrepancy between theory and experiment as a consequence of the viscous freezing of the vortex structure when field-cooling from the vortex liquid phase towards the glassy vortex phase. In order to be reliable, these studies on long-range vortex density fluctuations require the direct imaging of individual vortex positions in extended fields-of-view. Then, applying these hyperuniformity studies in order to infer information on the nature of the pinning centers present in superconducting samples relies on having extended and high-resolution snapshots with thousand of vortices or more, which is sometimes technically challenging.

## Supplementary Note 2

In order to calculate the local particle-particle interaction force for the structures nucleated in every studied medium, we have to consider the penetration depth at the freezing temperature $T_{\rm freez}$ at which disorder in the medium hinders the meandering of vortices in length-scales larger than $a_0$. This temperature is of the order of that at which pinning sets in, namely the irreversibility temperature $T_{\rm irr}$.[53,61] We measure the field dependence of $T_{\rm irr}$ by means of local Hall magnetometry techniques.[66] At a given field, $T_{\rm irr}$ is estimated from the onset of non-linearities in the magnetic response, namely at the temperature where $\mid T_{\rm h3} \mid$ overcomes the experimental noise level on cooling, see arrow in the inset to Fig. 1. Then data are inverted to obtain the $B_{\rm irr}$ as a function of temperature shown in Fig. 1. This figure shows the irreversibility line $B_{\rm irr}(T)$ for all samples studied in this work.

For samples in its pristine form and those with correlated disorder, the slope of $B_{\rm irr}$ is quite similar in a $T/T_{\rm c}$ scale (and also in a $T$ scale since $T_{\rm c}$ is similar for both sets of samples). The case of samples with extra point disorder generated by electron irradiation is different: the slope of $B_{\rm irr}$ is reduced concomitantly with a lowering of $T_{\rm c} = 66\,{\rm K}$.

The irreversibility lines for each sample are considered to obtain the value of $\lambda(T_{\rm freez} \approx T_{\rm irr})$ that enters into the vortex-vortex interaction force. We assume the temperature dependence $\lambda(T_{\rm freez}) = \lambda_{\rm ab}(0)/\sqrt{1-(T_{\rm freez}/T_{\rm c})^4}$ and consider $\lambda(0) = 180\,{\rm nm}$ for samples with correlated disorder and pristine,[53,65] and $\lambda_{\rm ab}(0) = 230\,{\rm nm}$ for samples with extra point disorder.[64] Extra point disorder introduced by electron irradiation produces a depletion in the superfluid density of the material and then $\lambda(0)$ increases. [64]

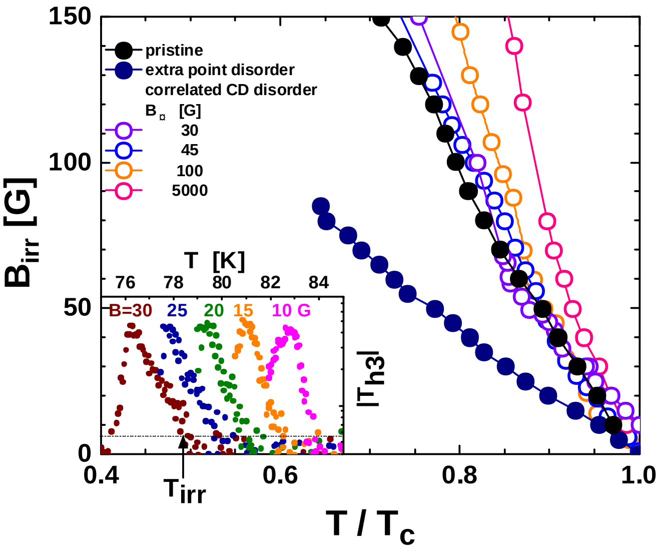


Figure 1. Irreversibility lines $B_{\rm irr}(T)$ for the $Bi_2Sr_2CaCu_2O_{8+\delta}$ samples studied in this work with point disorder (pristine and electron-irradiated) and correlated CD disorder (heavy-ion-irradiated). The matching fields $B_\Phi$ for the samples with correlated disorder are indicated. Inset: Temperature-evolution of the modulus of the third-harmonic signal $\mid T_{\rm h3} \mid$ obtained from ac magnetization measurements. Data for various fields are shown for the illustrative example of $B_\Phi = 30\,{\rm G}$. The irreversibility temperature $T_{\rm irr}$ is determined from the onset of non-linearities in the magnetic response, namely at the point indicated with an arrow where $\mid T_{\rm h3} \mid$ overcomes the experimental noise level (horizontal line) on cooling.

## Supplementary Note 3

The density of vortices in Figs. 1 (c) and (d) of the main text is equal to the matching field $B_\Phi = 30\,\mathrm{G}$ of the correlated CD pinning distribution. Then, in this case there is globally the same number of vortices and pinning sites. However, this does not mean that every vortex is located on top of a CD. This can be studied by comparing the pair correlation function for the experimentally observed vortex structure with that of a structure with the same vortex density but spatially arranged following a poissonian distribution as that of the CD landscape.[21] The insets to Fig. 2 show a zoom-in of the vortex structure observed experimentally (top panel) and of the distribution of correlated pinning centers following a poissonian distribution (bottom panel) for both structures with the same global density. This comparison shows that the vortex structure nucleated in samples with correlated disorder for $B/B_\Phi = 1$ is disordered, but particles do not follow a poissonian distribution in the sample: The $g(r)$ of the experimental structure presents clear peaks at distances corresponding to the first, second and third neighbors of a hexagonal lattice, whereas that of CD poissonian distribution fluctuates around 1 at all $r/a_0$. Then, the experimental structure does not mimic the correlated pinning distribution and moreover, presents a hyperuniform disorder as we reported previously.[46] This implies that, at some particular locations, since the spatial distribution of CD is poissonian, some defects are closer than $a_0$ and locating vortices on these particular pins is energetically unfavorable. This lack of mimicking of the pinning landscape by the particles will also hold in the case of poissonian distributed point pinning centers, given the gain in pinning energy is even smaller in this latter case as to balance the loss of elastic energy. Therefore, studying the $g(r)$ of elastic structures at densities commensurate with that of correlated disorder ($B/B_\Phi = 1$) does not seem a promising way for ascertaining whether disorder in the media is correlated or point-like.

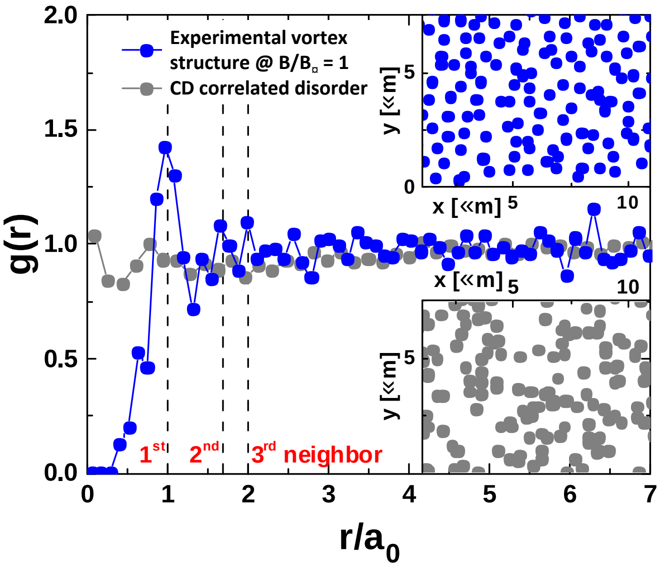


Figure 2. Pair correlation functions for the experimental vortex structure nucleated at $B/B_\Phi = 1$ (blue curve) in the $Bi_2Sr_2CaCu_2O_{8+\delta}$ sample with correlated disorder with $B_\Phi = 30\,\mathrm{G}$, and for a random Poissonian distribution of CD correlated disorder with the same density than that of vortices (gray curve). Top inset: vortex positions observed experimentally. Bottom inset: positions of CD following a poissonian distribution with a density equal to the matching field of $B_\Phi = 30\,\mathrm{G}$.

## Supplementary Note 4

In the fields of view shown in Fig. 1 of the main text, no topological defects are observed in the samples with point disorder (pristine and electron irradiated) at $B = 30\,\mathrm{G}$. In contrast, there are plenty of non-sixfold coordinated vortices in samples with correlated disorder (heavy-ion irradiated): 54 % at the same magnetic induction. We studied larger fields-of-view containing up to 15000 vortices at every $B$ in order to have statistics on the field-dependence of the density of topological defects, $\rho_{\mathrm{def}}$, see results in Fig. 3(a). For point disorder, at low magnetic inductions the structure is policrystalline, but on increasing field the size of crystallites enhances and for fields $B > 15\,\mathrm{G}$ becomes single-crystalline. This produces a decrease in $\rho_{\mathrm{def}}$ on increasing $B$. In pristine samples $\rho_{\mathrm{def}}$ decreases from 48 % at 4 G to 1.1 % at 28 G. In the case of the electron irradiated sample, $\rho_{\mathrm{def}}$ dropped from 33 % to 0.3 % at the same $B$.[45] In contrast, when nucleated in a sample with correlated disorder, the vortex structure is amorphous at low fields and presents small crystallites with less than 150 vortices on increasing field. This results in large values of $\rho_{\mathrm{def}} > 40\,\%$ up to 100 G. The inset to Fig. 3 (a) shows $\rho_{\mathrm{def}}$ as a function of $B/B_\Phi$ for the vortex structures nucleated in samples with CD that we study here and published data obtained in other samples for comparison.[34] For densities $B/B_\Phi < 2$ the vortex structure is amorphous and $\rho_{\mathrm{def}} \sim 50\,\%$. On further increasing $B/B_\Phi$ the vortex structure becomes policrystalline and $\rho_{\mathrm{def}}$ decreases systematically down to $\sim 13\,\%$ at $B/B_\Phi \sim 16$. This figure shows that at high vortex densities $\rho_{\mathrm{def}}$ is quantitatively different for point than for correlated disorder, but at low densities $\rho_{\mathrm{def}} \sim 50\,\%$ in both cases.

Another magnitude that can be quantified from real-space imaging of elastic structures nucleated in disordered media is the density fluctuation at first-neighbors distance, obtained from the spatially inhomogeneous distribution of first-neighbor distances $a$. In structures nu-

cleated in a media with point disorder, a rather uniform density of vortices is observed. In contrast, a tendency to vortex clustering is usually observed in structures nucleated in samples with strong and dilute correlated disorder. This difference in particle density-fluctuations at first-neighbor distance can be quantified by computing the standard deviation of the spatial distribution of first-neighbor distances, $SD$. Examples of the probability density function of first-neighbor distances, $a$, normalized by its mean value $a_0$, are shown in the inset to Fig. 3 (b). This figure shows data of structures nucleated at 30 G in samples with point and correlated CD disorder, the distribution of the latter being noticeably wider than that of the former.

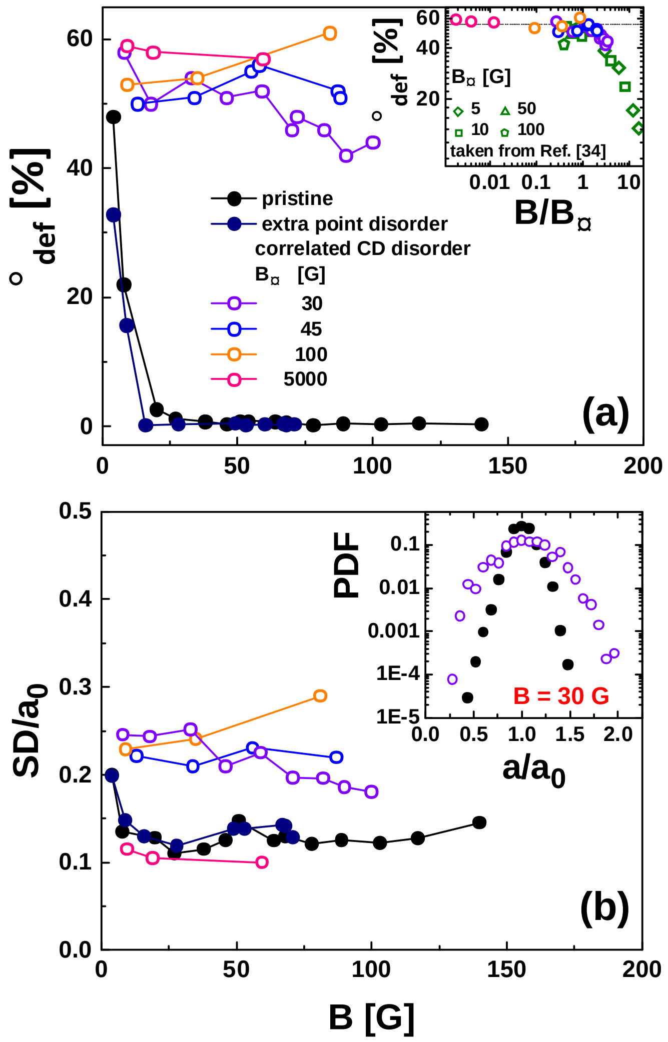


Figure 3. (a) Density of topological defects as a function of vortex density $B$ for vortex structures nucleated in $Bi_2Sr_2CaCu_2O_{8+\delta}$ samples with point and correlated disorder. Samples with point disorder are pristine and irradiated with electrons, whereas correlated disorder is produced by CD generated by heavy-ion irradiation resulting in different defect density quantified by the matching field $B_\Phi$. Inset: density of defects in the vortex structure nucleated in samples with correlated disorder as a function of $B/B_\Phi$ for the samples studied here and data for Pb-irradiated samples from the literature. (b) Standard deviation of the first-neighbors distances, $SD$, normalized by the mean lattice spacing, $a_0$, for the samples studied here. Inset: Probability density function of the normalized first-neighbors distance $a/a_0$ for a vortex density of 30 G nucleated in pristine and heavy-ion irradiated ($B_\Phi = 30$ G) samples.

The main panel of Fig. 3 (b) depicts the evolution of the normalized magnitude $SD/a_0$ as a function of vortex density $B$ for all the studied cases. Curves for structures nucleated in samples with point disorder, irrespective of its magnitude (pristine or extra disorder generated by electron-irradiation), are packed at low $SD/a_0$ values of roughly 0.2 at very low densities and 0.13 at intermediate vortex densities. Data for structures nucleated in samples with dilute correlated disorder, $B_\Phi = 30 - 100$ G in our case, are also packed around a larger value of $SD/a_0$ varying roughly between 0.2-0.3 in the whole studied vortex density. This discrepancy in the vortex density fluctuations at first-neighbor distance is presumably due to difference in the density and magnitude of pinning centers, being dense and weak for samples with point disorder and diluted and strong for samples with CD. In the latter case, the gain in pinning energy when trying to mimic the CD landscape can account for the larger fluctuations in $a$. The structures nucleated at $B \ll B_\Phi$ for a dense distribution of pins with $B_\Phi = 5000$ G seem to follow a different phenomenology: The values of $SD/a_0$ measured in this case are close to those of samples with point disorder. This can be explained considering that the density of pins, even they are correlated and strong, is between 80 to 400 times larger than the particle density and a vortex can profit from a pinning center with no need of generating large $a$ fluctuations. Then, the magnitude and field-evolution of $SD/a_0$ is not an unambiguous indicative of disorder being point or correlated in nature, but can give a hint on the media presenting dilute correlated disorder if its magnitude is larger than 20 % for intermediate vortex densities. Nevertheless, this criteria is not very qualitative nor sufficiently clear to apply.
